# Supplementary material for: Enhanced interlayer interactions in Ni-doped MoS$_2$, and structural and electronic signatures of doping site
Source: arXiv:2008.04301 ancillary file (2021-06-30)
Supplement: Supplementary file 1 [file SI.pdf]

# Supporting Information: Enhanced interlayer interactions in Ni-doped $MoS_2$, and structural and electronic signatures of doping site

Rijan Karkee, Enrique Guerrero, and David A. Strubbe*

*Department of Physics, University of California, Merced, Merced, CA 95343*

E-mail: dstrubbe@ucmerced.edu

**Table S1: Doping formation energy (eV) from LDA for Mo substitution under Mo-rich (S-rich) conditions.**

| Supercell | 2H | 3R | 1H |
|---|---|---|---|
| 1×1×1 | 2.76 (-0.30) | 2.78 (-0.27) | - |
| 2×2×1 | 4.52 (1.46) | 4.52 (1.47) | 4.65 (1.71) |
| 3×3×1 | 4.80 (1.74) | 4.64 (1.59) | 4.91 (1.97) |
| 4×4×1 | 4.71 (1.65) | 4.71 (1.66) | 4.92 (1.98) |
| 1×1×2 | 2.84 (-0.22) | - | |
| 1×1×3 | 2.88 (-0.18) | - | |
| 1×1×4 | 2.92 (-0.14) | - | |
| 2×2×2 | 4.37 (1.31) | - | |
| 2×2×3 | 4.38 (1.32) | - | |
| 2×2×4 | 4.38 (1.32) | - | |
| 3×3×2 | 4.78 (1.72) | - | |
| 4×4×2 | 4.80 (1.74) | - | |

**Table S2: Doping formation energy (eV) from LDA for S substitution under Mo-rich (S-rich) conditions.**

| Supercell | 2H | 3R | 1H |
|---|---|---|---|
| 1×1×1 | 0.88 (2.41) | 1.32 (2.85) | 1.89 (3.36) |
| 2×2×1 | 2.02 (3.55) | 1.99 (3.52) | 2.35 (3.82) |
| 3×3×1 | 1.96 ( 3.49) | 1.93 (3.46) | 2.27 (3.74) |
| 4×4×1 | 1.96 (3.49) | 2.04 (3.57) | 2.27 (3.74) |
| 1×1×2 | 0.95 (2.48) | - | |
| 1×1×3 | 0.99 (2.52) | - | |
| 1×1×4 | 1.03 (2.56) | - | |
| 2×2×2 | 1.90 (3.43) | - | |
| 2×2×3 | 1.90 (3.43) | - | |
| 2×2×4 | 1.90 (3.43) | - | |
| 3×3×2 | 1.97 (3.50) | - | |
| 4×4×2 | 1.97 (3.50) | - | |

**Table S3: Doping formation energy (eV) from LDA per Ni for intercalations in 2H.**

| Supercell | Tetrahedral | Octahedral |
|---|---|---|
| 1×1×1 | 0.28 | 1.26 |
| 2×2×1 | 0.18 | 1.19 |
| 3×3×1 | 0.18 | 1.27 |
| 4×4×1 | 0.20 | 1.29 |
| 1×1×2 | 0.26 | 1.01 |
| 1×1×3 | 0.26 | 1.05 |
| 1×1×4 | 0.26 | 1.07 |
| 2×2×2 | 0.19 | 1.21 |
| 2×2×3 | 0.19 | 1.21 |
| 2×2×4 | 0.19 | 1.22 |
| 3×3×2 | 0.18 | 1.28 |
| 4×4×2 | 0.19 | 1.28 |
| 1×1×1 (with 2 Ni) | 0.25 | - |
| 2×2×1 (with 2 Ni) | 0.17 | - |

**Table S4: Doping formation energy (eV) from LDA in intercalations of 3R.**

| Supercell | Mo/S-atop tetrahedral | Hollow/S-atop tetrahedral | Trigonal pyramidal |
|---|---|---|---|
| 1×1×1 | 0.34 | 0.85 | - |
| 2×2×1 | 0.22 | 0.80 | 0.75 |
| 3×3×1 | 0.23 | 0.81 | 0.75 |
| 4×4×1 | 0.25 | 0.82 | 0.75 |

**Table S5: Doping formation energy (eV) from LDA for adatoms on 1H.**

| Supercell | Mo–atop | S–atop | Hollow |
|---|---|---|---|
| 1×1×1 | 1.19 | 2.41 | 1.76 |
| 2×2×1 | 1.46 | 3.61 | 1.77 |
| 3×3×1 | 1.45 | 3.58 | 1.74 |
| 4×4×1 | 1.45 | 3.57 | 1.73 |

**Table S6: Extrapolated doping formation energy (eV) from LDA, for the low-concentration limit as a function of doping site and phase. Linear extrapolations are from the smallest two calculated values of $1/V$ (Fig. 5), which may not be fully converged in all cases. 3R has less sensitivity along the $z$-direction (due to larger $c$-parameter) and convergence is achieved with flat slope (shown in Fig. S1). The $N \times N \times 1$ series is similar between 2H and 3R and hence we expect the same for rest of the series. For monolayer 1H, we only have $N \times N \times 1$ due to vacuum along $z$-direction. Doping formation for substitutions is reported for Mo-rich (S-rich) conditions.**

a) 2H

| Doping type | $N \times N \times 2$ | $N \times N \times 1$ | $2 \times 2 \times N$ | $1 \times 1 \times N$ |
|---|---|---|---|---|
| **Mo subs.** | 4.82 (1.76) | 4.60 (1.54) | 4.39 (1.33) | 3.08 (0.02) |
| **S subs.** | 1.98 (3.51) | 1.98 (3.51) | 2.12 (3.65) | 1.15 (2.68) |
| **Tetrahed. intercal.** | 0.21 | 0.22 | 0.37 | 0.28 |
| **Octahed. intercal.** | 1.29 | 1.32 | 1.23 | 1.12 |

b) 3R and 1H, all $N \times N \times 1$

| Doping type | 3R | Doping type | 1H |
|---|---|---|---|
| **Mo subs.** | 4.78 (1.73) | **Mo subs.** | 4.95 (2.01) |
| **S subs.** | 2.16 (3.69) | **S subs.** | 2.28 (3.75) |
| **Trigonal pyramidal** | 0.75 | **Mo-atop ad.** | 1.42 |
| **Mo/S-atop tetrahed.** | 0.28 | **S-atop ad.** | 3.55 |
| **Hollow/S-atop tetrahed.** | 0.83 | **Hollow ad.** | 1.70 |

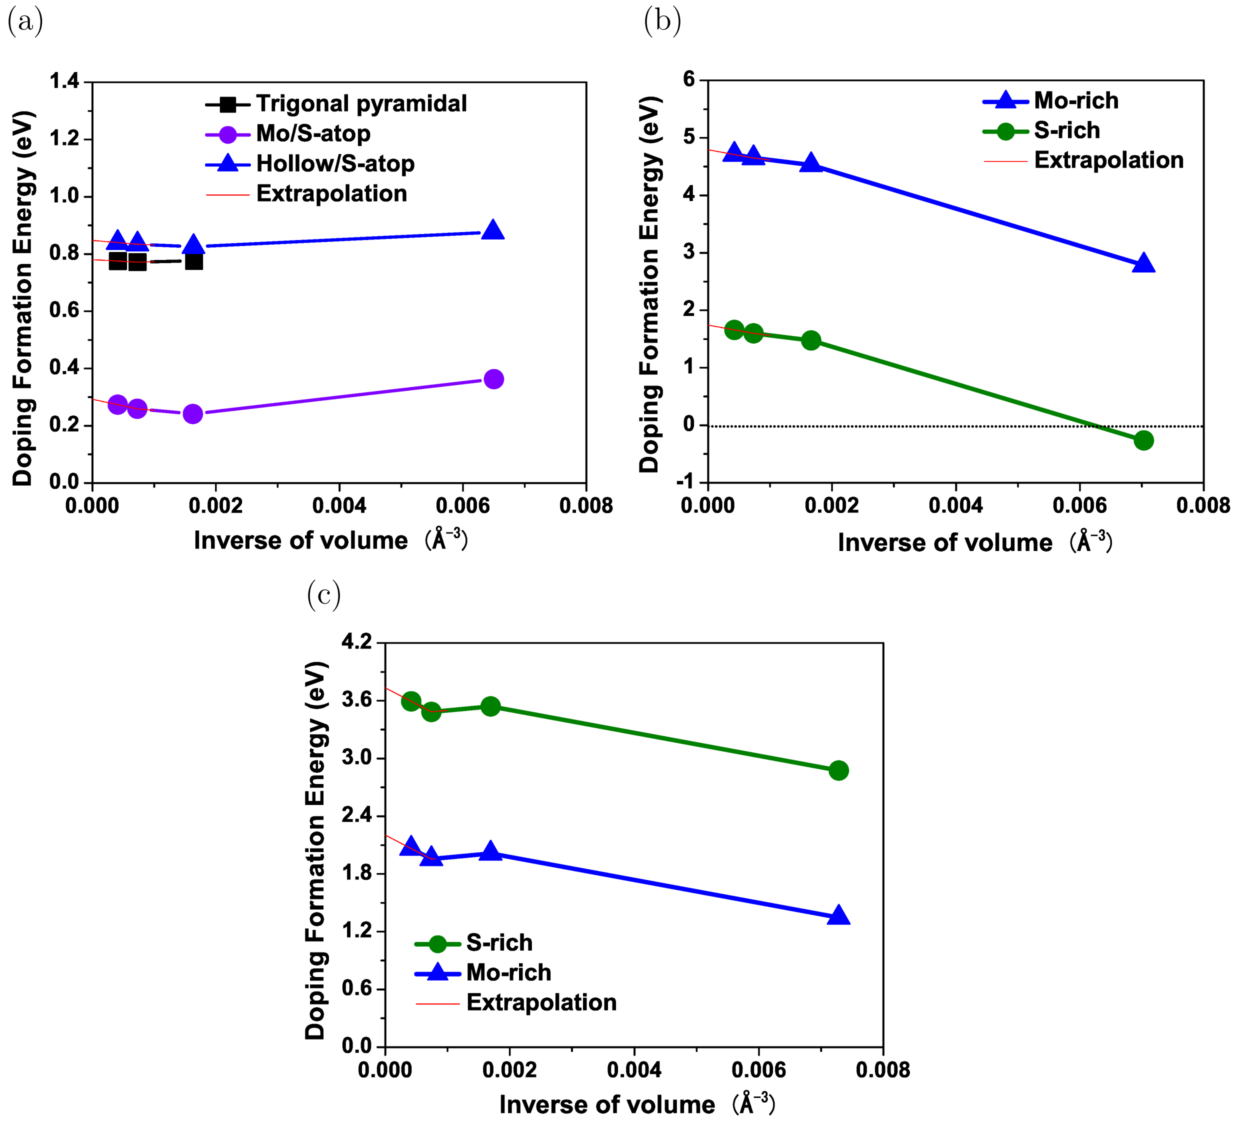


Figure S1: Doping formation energy from LDA of 3R-$MoS_2$: a) intercalations, b) Mo substitution under Mo-rich and S-rich conditions (where it can be negative), and c) S substitution under S-rich and Mo-rich conditions. Trigonal pyramidal for high concentration ($1 \times 1 \times 1$ supercell) is not shown because it is unstable.

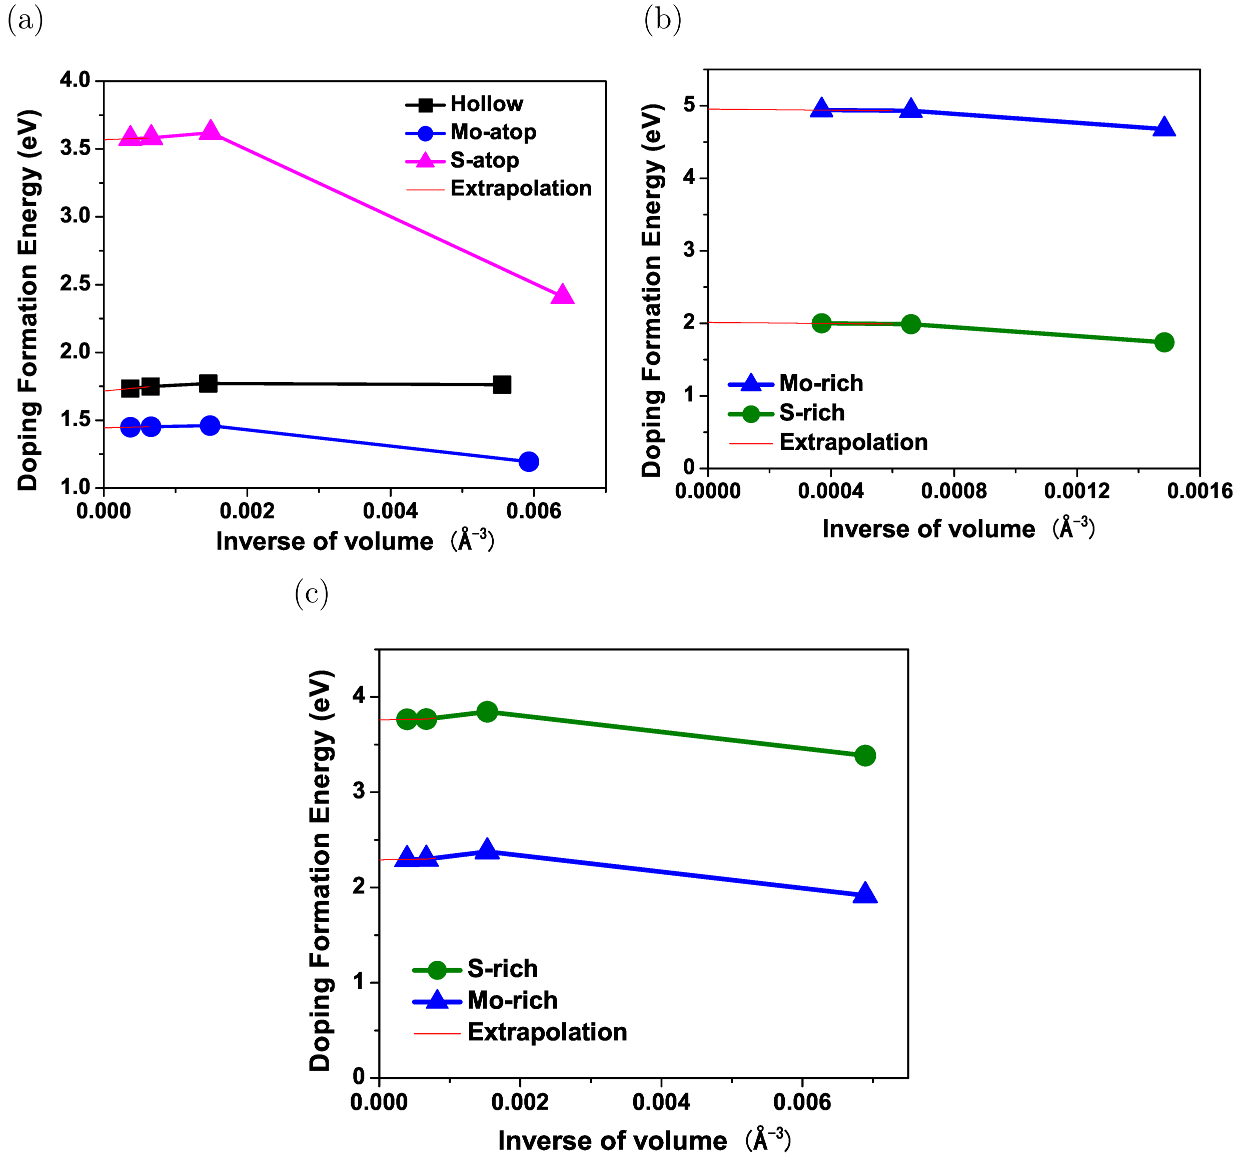


Figure S2: Doping formation energy from LDA of 1H-$MoS_2$: a) adatoms, b) Mo substitution under Mo-rich and S-rich conditions, and c) S substitution under S-rich and Mo-rich conditions.

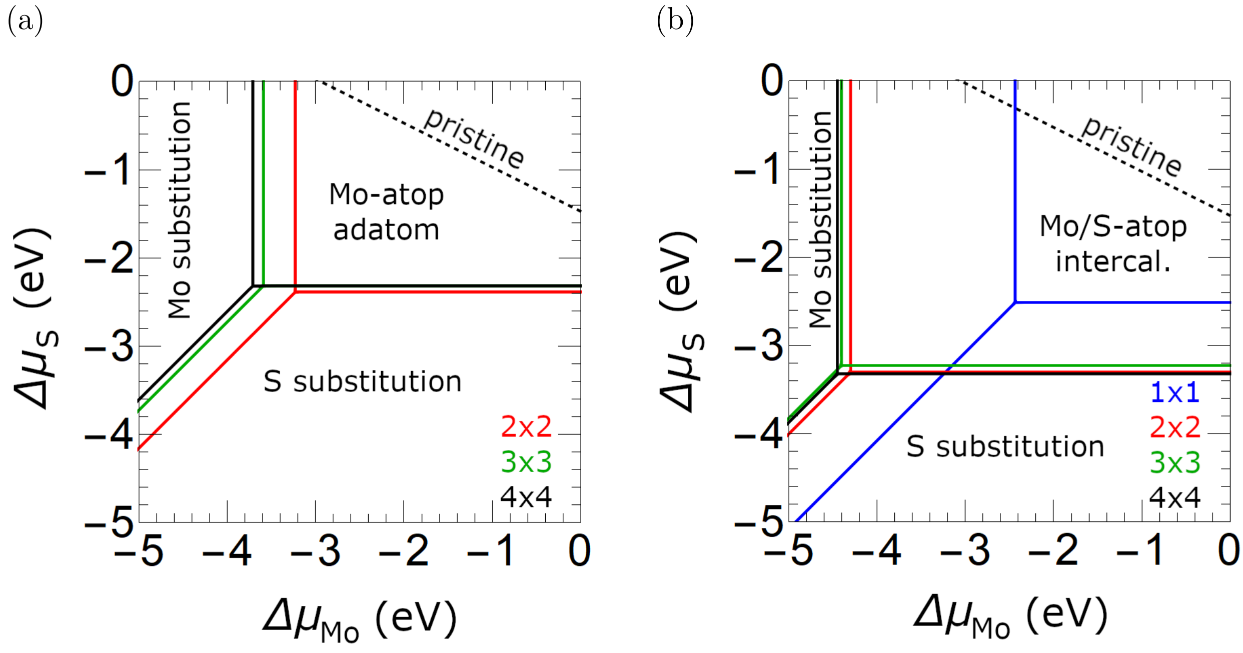


Figure S3: Phase diagrams from LDA for a) 1H and b) 3R polytypes, indicating the stable doping site as a function of Mo and S chemical potentials, as in Ref. 17. The pristine phase is stable in the triangle above and to the right of the dotted line.

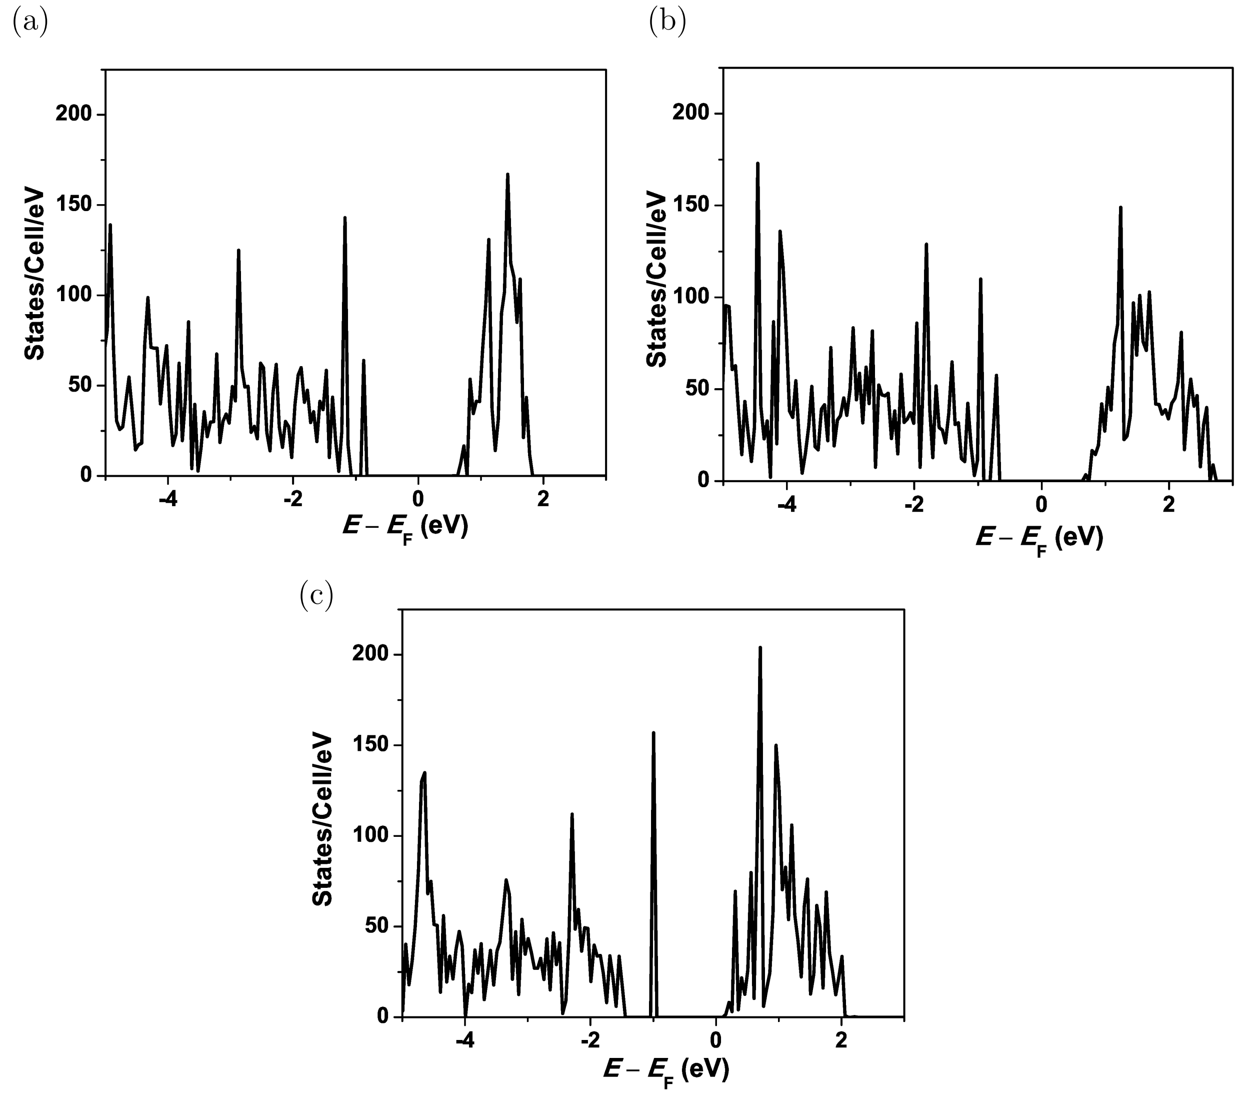


Figure S4: Electronic density of states from PBE+GD2 for 1H 4×4×1 structures for a) Mo–atop, b) hollow site, and c) S–atop. A broadening of 0.001 eV was used to show in-gap states.

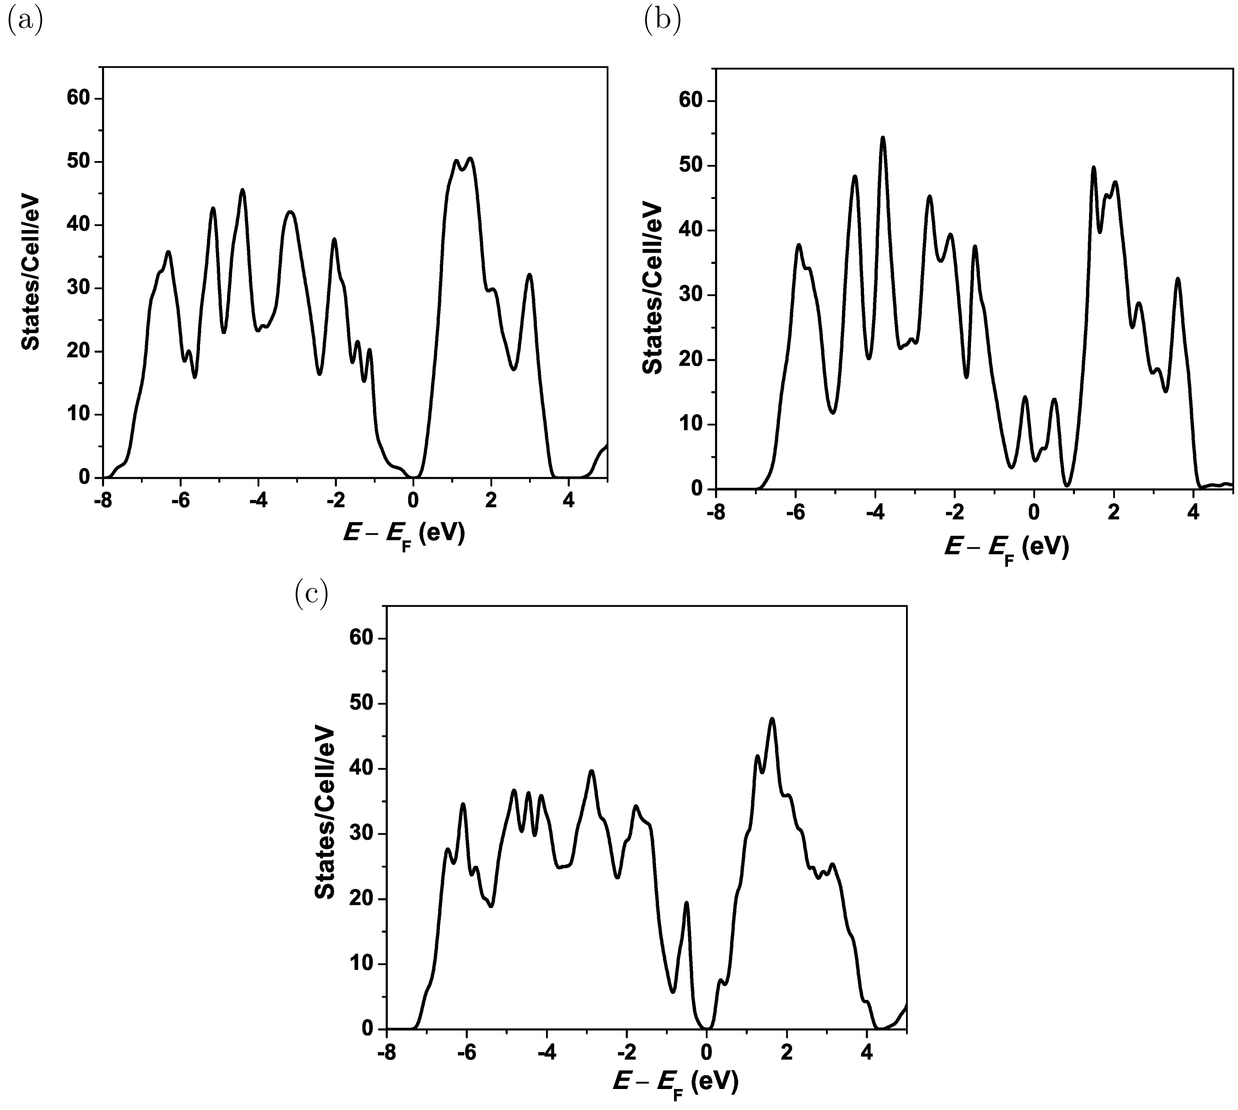


Figure S5: Electronic density of states from PBE+GD2 for 3R 2×2×1 structures: a) Mo/S-atop tetrahedral intercalation, b) Mo substitution, and c) S substitution.

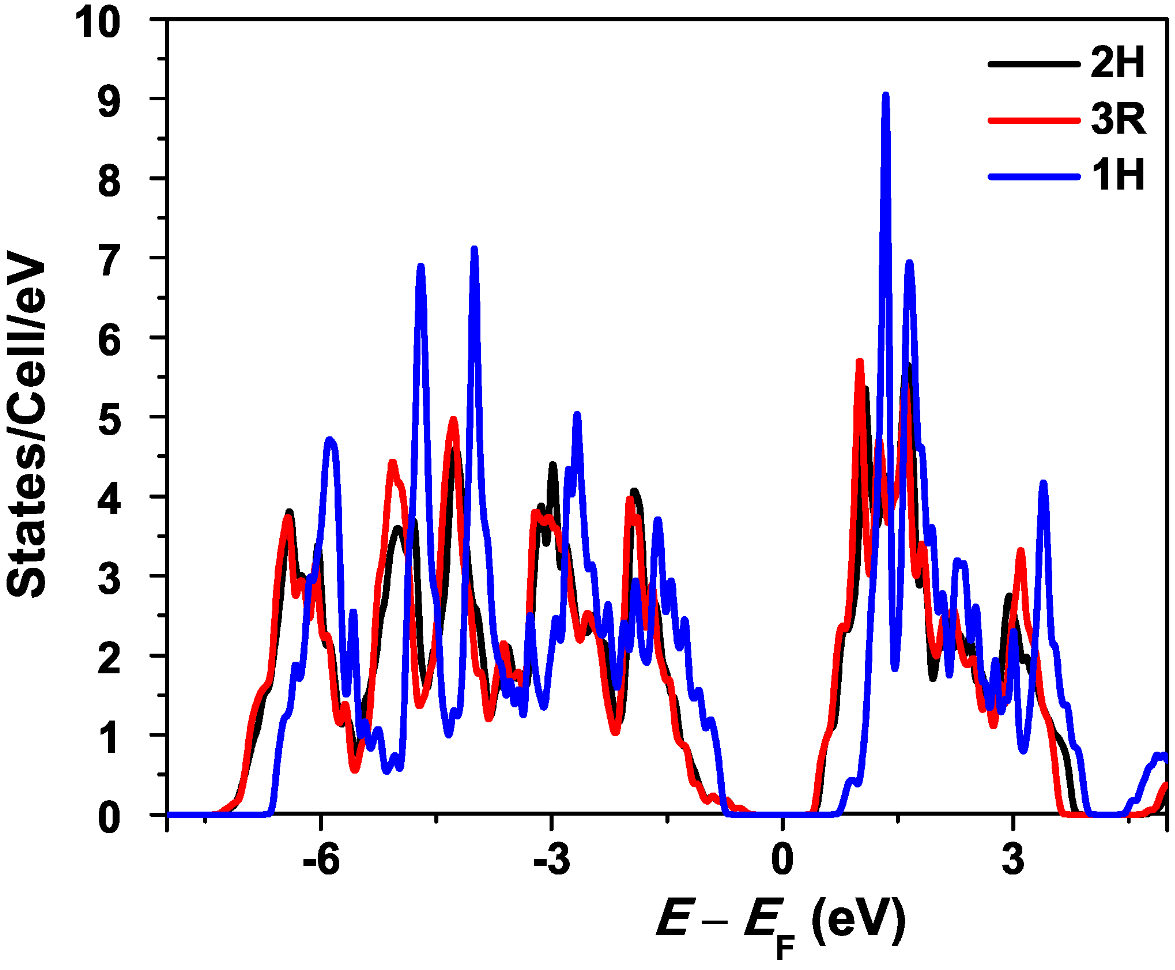


Figure S6: Electronic density of states from PBE+GD2 for pristine $MoS_2$ polytypes, per $MoS_2$ unit. $E_F$ is taken as the mid-point of band gap in each case. A broadening of 0.002 eV was used to distinctly show gaps for each case.
